# Supplementary material for: Multi-reference protocol for (auto)ionization spectra: application to molecules
Source: arXiv:1912.04139 source file (2019-12-09)
Supplement: Supplementary file 1 [file supplement.pdf]

**Supplementary material:**

# Multi-reference protocol for (auto)ionization spectra: application to molecules

Gilbert Grell[a] and Sergey I. Bokarev

*Institut für Physik, Universität Rostock, Albert-Einstein-Str. 23-24, 18059 Rostock, Germany*

(Dated: December 7, 2019)

In this contribution we present the application of the spherically averaged continuum model to the evaluation of molecular PES and AIS / AES

[a] gilbert.grell@uni-rostock.de

## I. ADDITIONAL DATA

Herein we present additional results for the methane and oxygen photoelectron spectrum (PES) and resonant Auger electron spectrum (RAES).

### A. Methane $CH_4$

Below we show the PES and RAES of $CH_4$ obtained with continuum orbitals corresponding to different approximations to the spherically averaged potentials than the spherically averaged direct potential $V_f^{\mathrm{J}}(r)$ that has been used throughout the main text. First, the dependence of the methane PES at 282.2 eV on the continuum orbital approximations is illustrated in Fig. S1. Therein the PES have been obtained using the same quantum chem-

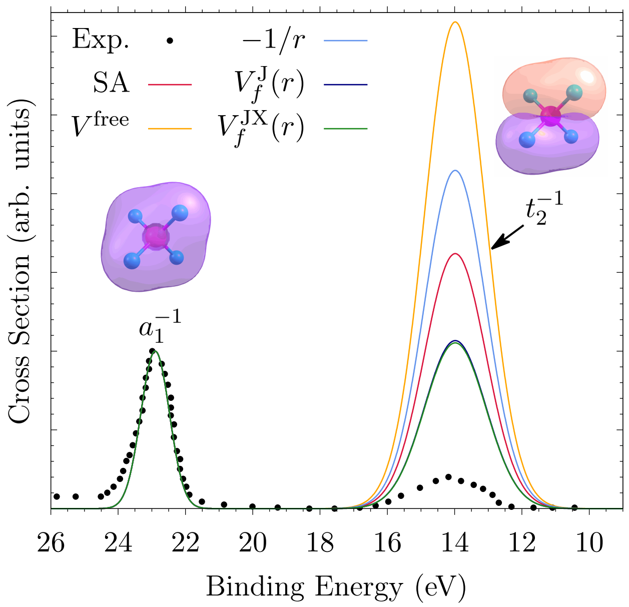


Figure S1. Theoretical results for the 282.2 eV methane valence PES obtained with continuum orbitals corresponding to the indicated potential models.[1] The experimental reference has been digitized from Kivimaeki et al.[2] In addition, the normalized Dyson orbitals for the respective $a_1^{-1}$ and $t_2^{-1}$ features are shown. As in the main text, the spectra have been aligned to the experimentally obtained value for the $a_1^{-1}$ ionization potential of 22.90 eV[3]. The broadening is detailed in Table S1.

istry (QC) protocol, as described in the main text. However, results corresponding to the free-particle, effective Coulomb, direct, and direct-exchange potentials, $V^{\mathrm{free}}$, $-1/r$, $V_f^{\mathrm{J}}(r)$, and $V_f^{\mathrm{JX}}(r)$, introduced in Ref. 1, are compared. Note that the $V_f^{\mathrm{J}}(r)$ result corresponds to the PES shown in Fig 1. of the main text. Further, results obtained in sudden approxima-

tion (SA)[4], neglecting the continuum orbital treatment entirely, are depicted as well. In SA, the cross section of each transition is approximated by the squared norm of the respective Dyson orbital: $\sigma_{g\alpha} \approx ||\Phi_{g\alpha}||^2$. Note, that at this energy none of the potential models that have been devised by reproduces the correct intensity ratio of $a_1^{-1}$ and $t_2^{-1}$ features. However, the $V_f^{\mathrm{JX}}(r)$ and $V_f^{\mathrm{J}}(r)$ potentials yield the closest agreement with the experimental data.

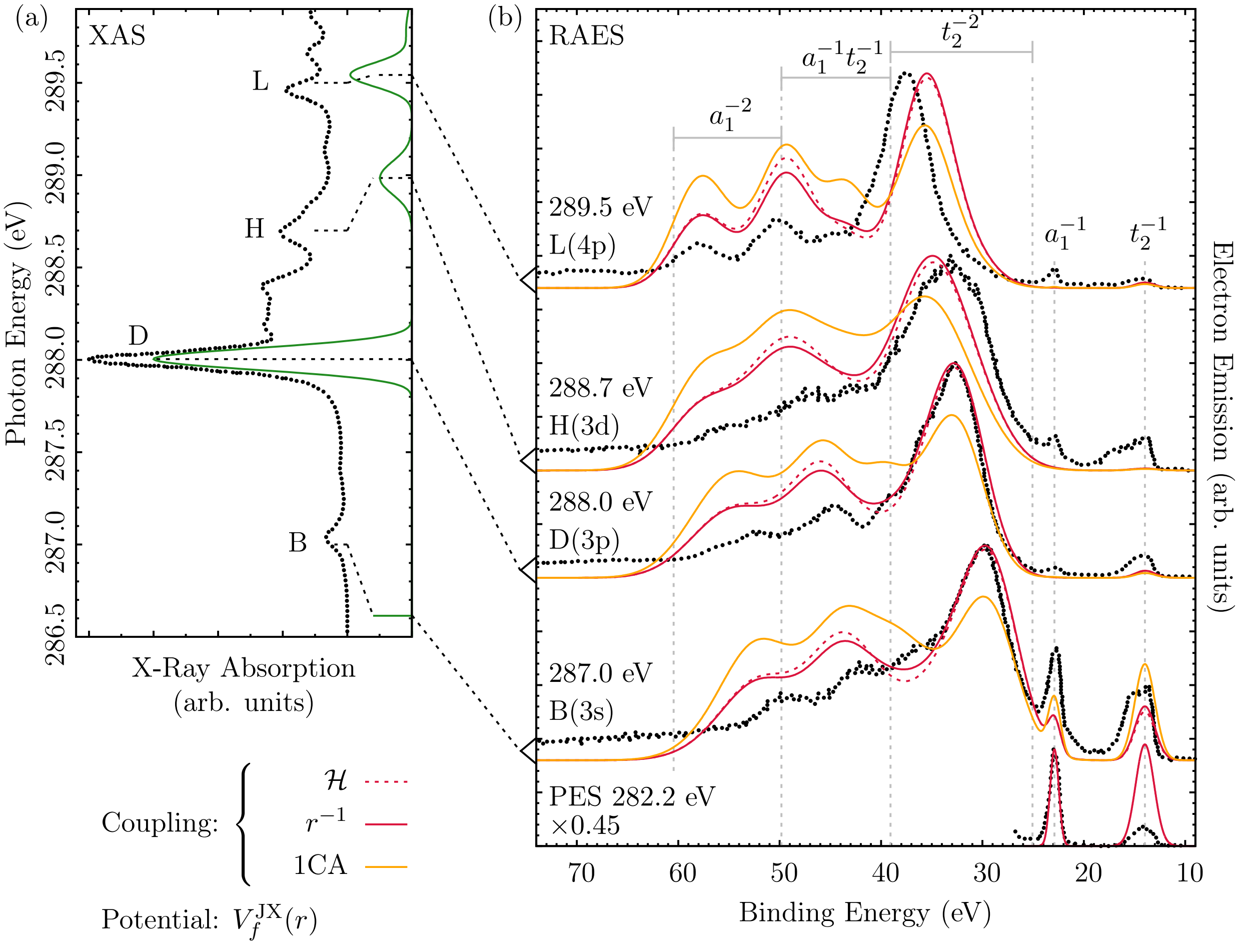


Figure S2. All experimental data (dotted) have been digitized from Kivimaeki et al.[2] (a) Calculated (green) and experimental XAS of methane at the carbon K-edge. The dipole-forbidden $3s(a_1)$ excitation is indicated by a single stick. The assignment of the experimental spectrum[5,6] is connected to the corresponding calculated core-excited states of $CH_4$. (b) For each resonance depicted in (a) the RAES calculated using continuum orbitals corresponding to the direct-exchange $V_f^{\mathrm{JX}}(r)$ potential and the indicated couplings are shown together with the measured results. The $\mathcal{H}$, $r^{-1}$, and 1CA spectra for one resonance have been normalized with the same constant. The respective calculated carbon Rydberg contributions are given in paranthesis for each resonance. Further, spectral regions have been assigned to different valence hole states of $CH_4^+$ (gray). The experimental and theoretical valence PES obtained at a photon energy of 282.2 eV are shown as well. Shifts: see main text; broadenings: see Table S1.

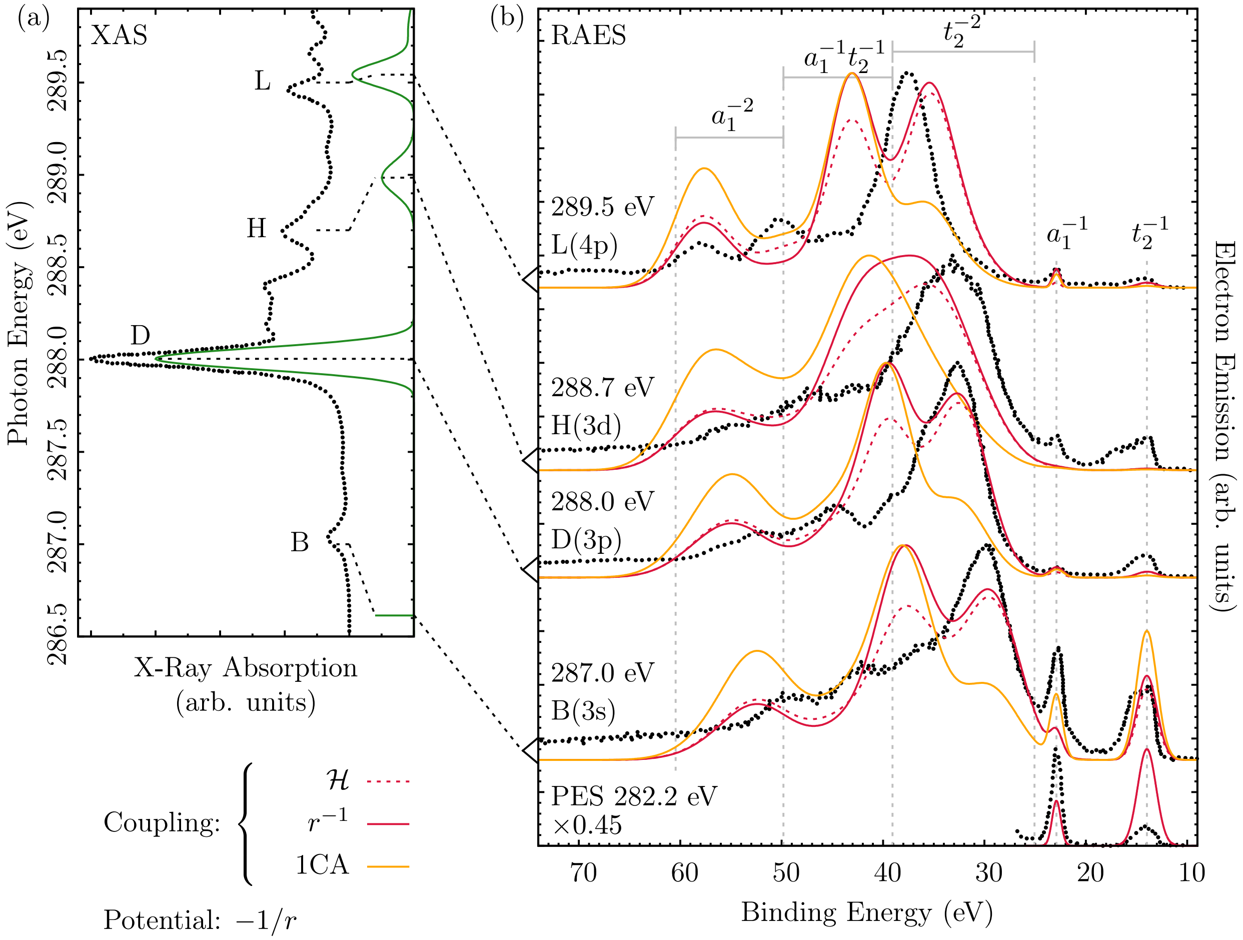


Figure S3. All experimental data (dotted) have been digitized from Kivimaeki et al.[2] (a) Calculated (green) and experimental XAS of methane at the carbon K-edge. The dipole-forbidden $3s(a_1)$ excitation is indicated by a single stick. The assignment of the experimental spectrum[5,6] is connected to the corresponding calculated core-excited states of $CH_4$. (b) For each resonance depicted in (a) the RAES calculated using continuum orbitals corresponding to the effective Coulomb potential $-1/r$ and the indicated couplings are shown together with the measured results. The $\mathcal{H}$, $r^{-1}$, and 1CA spectra for one resonance have been normalized with the same constant. The respective calculated carbon Rydberg contributions are given in paranthesis for each resonance. Further, spectral regions have been assigned to different valence hole states of $CH_4^+$ (gray). The experimental and theoretical valence PES obtained at a photon energy of 282.2 eV are shown as well. Shifts: see main text; broadenings: see Table S1.

In Figs. S2 and S3, the RAES and PES results obtained with continuum orbitals corresponding to the spherically averaged direct-exchange $V_f^{\mathrm{JX}}(r)$ and effective Coulomb potential, $-1/r$, approaches, are depicted. For a better visual correspondence with Fig. 1 in the main text, which depicts data obtained with the spherically averaged direct potential $V_f^{\mathrm{J}}(r)$, the same format has been chosen and the XAS are repeated as well. Note that in

comparison to the $V_f^{\mathrm{J}}(r)$ results in the main text, Fig. 1, the $V_f^{\mathrm{JX}}(r)$ RAES are slightly worse, leading to a more pronounced overestimation of the high binding energy tail (40-60 eV). The decay spectra obtained with the $-1/r$ potential, modelling the molecule as a point charge, however, deviate strongly from the $V_f^{\mathrm{J}}(r)$ and $V_f^{\mathrm{JX}}(r)$ ones. In particular the $a_1^{-1}t_2^{-1}$ region is strongly overestimated, leading to a shift of the main maximum towards the $a_1^{-1}t_2^{-1}$ part of the spectra. The 1CA enhances this characteristics even more.

## B. Oxygen $O_2$

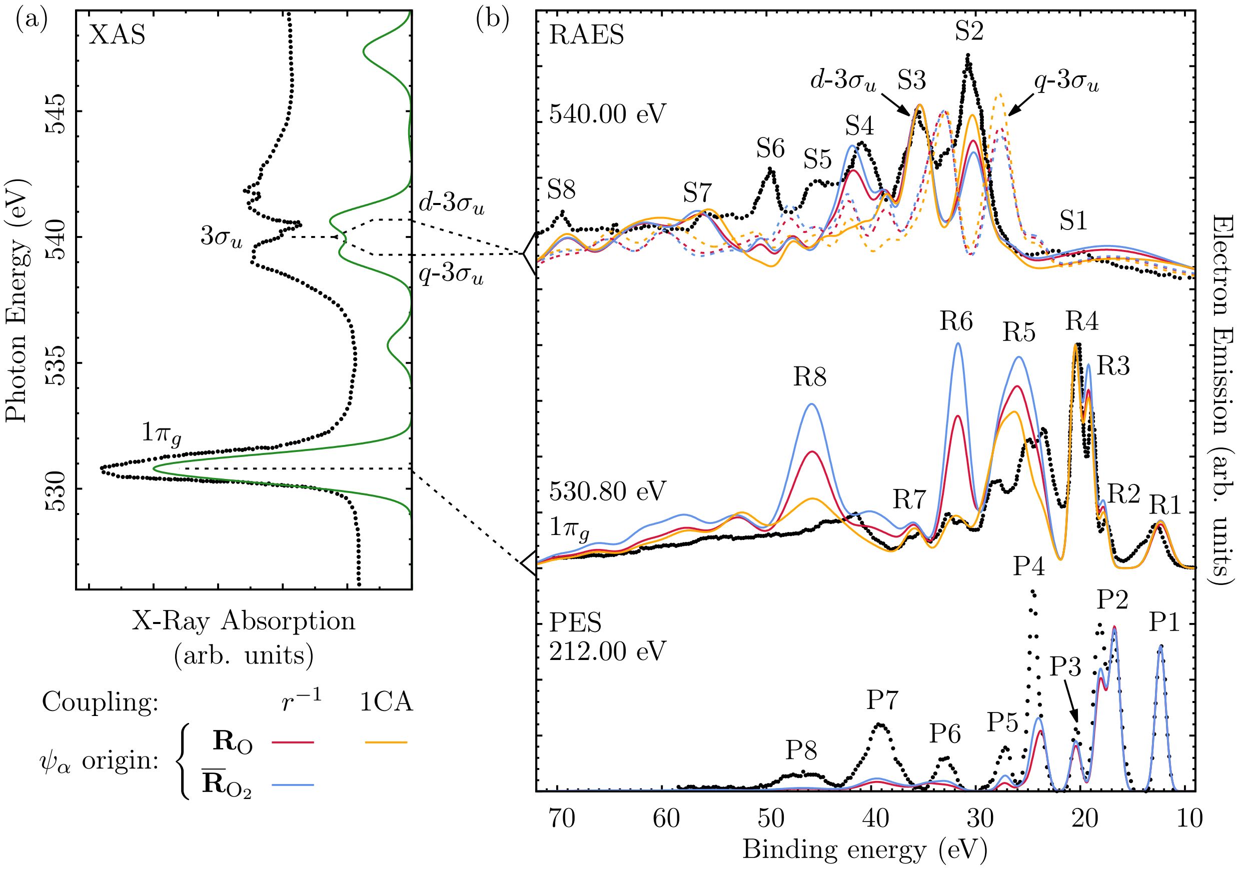


Figure S4. (a) Calculated (green) and experimental[7] (dotted) K-edge XAS of $O_2$. The theoretically obtained $1\pi_g$, $q$-$3\sigma_u$, and $d$-$3\sigma_u$ resonance positions are connected to the experimental excitation energies that have been used to obtain the respective RAES. In panel (b) the simulated PES and RAES are compared to the measurements by Caldwell et al.[8] Note that due to the low monochromater resolution present in the experiment[8], the whole exchange split $3\sigma_u$ double peak is excited by the incoming radiation at 540 eV. Hence, the theoretical RAES obtained for the $q$-$3\sigma_u$ (dashed) and $d$-$3\sigma_u$ (solid) resonances are depicted together with the experimental one. The theoretical results employ the $V_f^{\mathrm{J}}(r)$ potential centered at $\mathbf{R}_\mathrm{O}$ or $\overline{\mathbf{R}}_{\mathrm{O}_2}$, respectively. Further, the $r^{-1}$ and 1CA couplings have been used. Shifts: see main text; broadenings: see Table S2.

To support the discussion in the main text, the theoretically obtained decay RAES for the $1\pi_g$, $q$-$3\sigma_u$, and $d$-$3\sigma_u$ resonances obtained with the $r^{-1}$ an 1CA coupling are compared against the respective experimental measurements[8] in Fig. S4. The spectra have been calculated with the spherically averaged direct potential approach $V_f^{\mathrm{J}}(r)$, as in the main text. Note that in particular the the $1\pi_g$ spectra are sensitive to the exclusion of the one-electron coupling terms within the approximate $r^{-1}$ coupling approach, which leads to larger overestimations of the features R5, R6, and R8 than observed for $\mathcal{H}$ coupling (Fig. 2 of the main text). In addition, the $r^{-1}$ $1\pi_g$ RAES show a stronger dependence on the continuum orbital origin, although the $\mathbf{R}_{\mathrm{O}}$ spectra still seems to agree better with the experiment than the $\overline{\mathbf{R}}_{\mathrm{O}_2}$ one.

## II. BROADENING PARAMETERS

Note that unless stated otherwise, the broadening parameters compiled herein for the respective XAS, PES and RAES of the $O_2$, $CH_4$, $NO_2$ and $C_4H_4N_2$ molecules have been applied to to produce the spectra in all respective figures that are shown herein and in the main text.

### A. Methane $CH_4$

The broadening parameters presented herein have been tuned such as to obtain the best representation of the respective experimental spectra that have been reported by Kivimäki et al. in Ref. 2. To construct the curve for the carbon K-edge XAS, the spectral regions corresponding to the D, H, and L features have been broadened with Gaussian profiles having respective full width at half maximums (FWHMs) parameters of 0.17 eV, 0.22 eV, and 0.21 eV. The PES, consisting of the $t_2^{-1}$ and $a_1^{-1}$ peaks have been obtained by broadening with a Gaussian FWHM of 1.75 eV and 1.15 eV, repsectively.

Table S1. Broadening parameters used for the $CH_4$ RAES corresponding to the indicated resonances. The respective binding energy intervals $\Delta\mathcal{E}_b$ and Gaussian FWHM parameters $\sigma$ are given in eV.

| B(3$s$) | | D(3$p$) | | H(3$d$) | | L(4$p$) | |
|---|---|---|---|---|---|---|---|
| $\Delta\mathcal{E}_b$ | $\sigma$ | $\Delta\mathcal{E}_b$ | $\sigma$ | $\Delta\mathcal{E}_b$ | $\sigma$ | $\Delta\mathcal{E}_b$ | $\sigma$ |
| 7.0-21.0 | 2.34 | 7.0-22.0 | 2.34 | 7.0-22.7 | 3.06 | 7.0-22.5 | 2.34 |
| 21.0-24.5 | 1.40 | 22.0-25.0 | 0.86 | 22.7-24.7 | 0.95 | 22.5-24.5 | 0.90 |
| 24.5-41.0 | 5.94 | 25.0-42.0 | 5.22 | 24.7-42.7 | 7.02 | 24.5-43.5 | 5.22 |
| 41.0-87.0 | 7.70 | 42.0-48.0 | 6.93 | 42.7-88.7 | 7.70 | 43.5-54.5 | 5.85 |
| | | 48.0-88.0 | 7.70 | | | 54.5-89.5 | 6.17 |

## B. Oxygen $O_2$

Table S2. Broadening parameters used for the $O_2$ XAS, PES, and RAES of the indicated resonances. The respective binding and excitation energy intervals $\Delta\mathcal{E}_b$, $\Delta\hbar\omega$, and Gaussian FWHM parameters $\sigma$ are given in eV.

| XAS | | PES | | $1\pi_g$ RAES | | $3\sigma_u$ RAES | |
|---|---|---|---|---|---|---|---|
| $\Delta\hbar\omega$ | $\sigma$ | $\Delta\mathcal{E}_b$ | $\sigma$ | $\Delta\mathcal{E}_b$ | $\sigma$ | $\Delta\mathcal{E}_b$ | $\sigma$ |
| 525-550 | 1.3 | 0.0-25.6 | 1.15 | 0.0-15.8 | 2.08 | 0.0-25.0 | 9.00 |
| | | 25.6-29.6 | 1.25 | 15.8-21.8 | 1.05 | 25.0-33.0 | 2.60 |
| | | 29.6-35.6 | 2.10 | 21.8-38.8 | 2.00 | 33.0-53.0 | 1.90 |
| | | 35.6-42.6 | 2.85 | 38.8-75.0 | 3.50 | 53.0-75.0 | 3.50 |
| | | 42.6-75.0 | 4.10 | | | | |

## C. Nitrogen dioxide $NO_2$

Table S3. Broadening parameters used for the $NO_2$ nitrogen K-edge XAS, PES, and RAES of the indicated resonances. The respective binding and excitation energy intervals $\Delta\mathcal{E}_b$, $\Delta\hbar\omega$ and Gaussian as well as Lorentzian FWHM parameters $\sigma$ and $\gamma$ are given in eV.

| XAS | | PES | | | $2b_1$ RAES at 402.86 eV | | $2b_1$ RAES at 403.73 eV | |
|---|---|---|---|---|---|---|---|---|
| $\Delta\hbar\omega$ | $\sigma$ | $\Delta\mathcal{E}_b$ | $\sigma$ | $\gamma$ | $\Delta\mathcal{E}_b$ | $\sigma$ | $\Delta\mathcal{E}_b$ | $\sigma$ |
| 395.0-402.0 | 0.83 | 0.0-12.3 | 1.325 | | 0.0-12.5 | 1.075 | 0.0-12.0 | 1.650 |
| 402.0-408.0 | 0.85 | 12.3-15.0 | 0.375 | | 12.5-16.0 | 0.275 | 12.0-15.5 | 0.275 |
| 408.0-410.3 | 0.53 | 15.0-18.2 | 0.925 | | 16.0-18.7 | 0.700 | 15.5-25.0 | 0.750 |
| 410.3-413.0 | 0.80 | 18.2-21.0 | 0.375 | | 18.7-20.6 | 0.650 | | |
| 413.0-425.0 | 5.00 | 21.0-21.5 | | 0.10 | 20.6-25.0 | 0.750 | | |
| | | 21.5-24.0 | 0.375 | | | | | |

## D. Pyrimidine $C_4H_4N_2$

Table S4. Broadening parameters used for the $C_4H_4N_2$ nitrogen K-edge XAS, PES, and RAES of the E6 resonance. The respective binding and excitation energy intervals $\Delta\mathcal{E}_b$, $\Delta\hbar\omega$, and Gaussian FWHM parameters $\sigma$ are given in eV.

| XAS | | PES | | E6 RAES | |
|---|---|---|---|---|---|
| $\Delta\hbar\omega$ | $\sigma$ | $\Delta\mathcal{E}_b$ | $\sigma$ | $\Delta\mathcal{E}_b$ | $\sigma$ |
| 397.00-399.50 | 0.650 | 0.0-12.5 | 0.60 | 0.0-23.0 | 0.75 |
| 399.50-400.45 | 0.550 | 12.5-15.0 | 1.00 | 23.0-28.0 | 2.05 |
| 400.50-401.80 | 0.750 | 15.0-16.2 | 0.85 | 28.0-34.0 | 4.25 |
| 401.80-408.00 | 0.625 | 16.2-19.8 | 1.50 | 34.0-56.0 | 11.35 |
| | | 19.8-22.5 | 0.95 | | |
| | | 22.5-28.0 | 1.70 | | |
| | | 28.0-56.0 | 3.10 | | |

## III. CARBON RYDBERG BASIS SET

This $(22s15p10d7f)/[7s5p3d2f]$ carbon Rydberg basis set has been used for the calculations regarding the $CH_4$ molecule, presented in the main text. It has been obtained in the following way: ANO-L exponents[9] have been supplemented by $(8s6p6d4f)$ Rydberg ones that have been generated according to the procedure in Ref. 10. The contraction coefficients have been obtained with the Genano module[11] of openMolcas.[12] Therein the density matrices of the ground and 82 lowest core-excited states of triplet carbon, as well 229 valence-excited states of doublet $C^+$, have been evenly averaged. Further, the active spaces $\mathrm{RAS}(6,1,1;2,3,31)$ and $\mathrm{RAS}(3,1,1;1,3,31)$ have been employed for C and $C^+$, respectively.

```
C S
      50557.501   0.0000554  -0.0000141   0.0000027  -0.0000017   0.0000002  -0.0000040   0.0000011
      7524.7856   0.0004352  -0.0001105   0.0000215  -0.0000130   0.0000018  -0.0000303   0.0000082
      1694.3276   0.0023206  -0.0005900   0.0001155  -0.0000698   0.0000100  -0.0001694   0.0000478
      472.82279   0.0098932  -0.0025273   0.0004923  -0.0002964   0.0000421  -0.0006817   0.0001815
      151.71075   0.0353011  -0.0091501   0.0017944  -0.0010852   0.0001553  -0.0026706   0.0007638
      53.918746   0.1045054  -0.0281065   0.0054752  -0.0032833   0.0004662  -0.0073974   0.0019298
      20.659311   0.2422650  -0.0710452   0.0140257  -0.0084527   0.0012177  -0.0213846   0.0063148
      8.3839760   0.3848476  -0.1383681   0.0273606  -0.0162794   0.0023069  -0.0342747   0.0082613
      3.5770150   0.3062910  -0.1767318   0.0382435  -0.0242088   0.0035259  -0.0707672   0.0229626
      1.5471180   0.0661304  -0.0014742   0.0021911  -0.0029828   0.0001661   0.0188711  -0.0144040
      0.6130130   0.0024826   0.5412056  -0.1238081   0.0785679  -0.0109681   0.1228821  -0.0120022
      0.2460680   0.0031351   0.5449053  -0.2861114   0.2201439  -0.0364162   0.8980101  -0.3429385
      0.0990870  -0.0001376   0.0299654  -0.0953666  -0.0125505   0.0061750  -1.0530334   0.5598165
      0.0346800   0.0001895   0.0080153   0.6640376  -0.7107209   0.1879168  -1.8684776   0.4972325
      0.0112533  -0.0003146  -0.0112501   1.1734161  -1.7229839   0.4642457   8.1033402  -7.4432742
      0.0058584   0.0006563   0.0240021  -1.6328915   4.9423058  -2.6760962 -13.9083785  22.7282046
      0.0033460  -0.0010909  -0.0451430   2.0757306  -4.1095298   2.2678469  16.3796464 -34.0610756
      0.0020484   0.0014954   0.0678743  -2.3625403   4.4587858  -0.9719151 -19.8538822  31.9166589
      0.0013236  -0.0016393  -0.0756157   2.4793296  -5.3949310   2.6242232  21.7800560 -26.9204925
      0.0008931   0.0013110   0.0592119  -2.0103029   4.1518568  -1.9756217 -16.9049493  21.5236943
      0.0006243  -0.0006532  -0.0294083   0.9996186  -2.0494694   1.0046833   8.3077284 -10.5946867
      0.0004495   0.0001484   0.0069038  -0.2185765   0.4701302  -0.2377670  -1.8957386   2.4266113
C P
      83.333155   0.0016902  -0.0002597   0.0000917  -0.0005516   0.0000552
      19.557611   0.0130821  -0.0019827   0.0007045  -0.0041427   0.0002019
      6.0803650   0.0604217  -0.0091431   0.0032355  -0.0194424   0.0019347
      2.1793170   0.1908470  -0.0296103   0.0105390  -0.0627215   0.0019610
      0.8651500   0.3738639  -0.0640343   0.0223935  -0.1447959   0.0222276
      0.3619440   0.4121089  -0.0880526   0.0316131  -0.2029583  -0.0345343
      0.1547400   0.1542508  -0.0381202   0.0138100  -0.0273092   0.2203000
      0.0654290  -0.0025207   0.1908643  -0.0446433   1.3202008  -0.5961192
      0.0229000   0.0046373   0.6889854  -0.5616569  -0.4186885   0.5047919
      0.0099882  -0.0004755   0.4573422  -0.1469174  -2.0066859   2.2560562
      0.0056894   0.0000637  -0.3786981   1.3767454   2.6949480  -6.5298946
      0.0034757  -0.0037287   0.1431867  -0.2367263  -1.6198145   5.4086750
      0.0022421   0.0031604  -0.0853635   0.2101873   0.8394500  -1.2277959
      0.0010548  -0.0001188   0.0164980  -0.0413206  -0.2019057   0.5871641
      0.0005596   0.0000729  -0.0043503   0.0105962   0.0531507  -0.1386142
C D
      1.9000000   0.0009482  -0.0077763   0.0040482
      0.6650000   0.0050964  -0.0332340   0.0167271
      0.2327500   0.0151610  -0.1801961   0.1012733
      0.0814630   0.0806746  -0.6635421   0.3425014
      0.0274457   0.3997480  -0.4010929  -0.0644277
      0.0142044   0.4478216   0.7300550  -0.6082779
      0.0080766   0.2124006  -0.2118336  -0.1330624
      0.0049272  -0.0279700   0.3318272   0.8205665
      0.0021371  -0.0111903   0.0462477   0.4680205
      0.0010717  -0.0006853   0.0066452  -0.0424699
```

```
C F
      1.2500000   0.0005086  -0.0003031
      0.5000000   0.0016939   0.0058104
      0.2000000   0.0212941   0.0102196
      0.0790699   0.1328150   0.2156680
      0.0357629   0.4158943   0.1920921
      0.0184778   0.3477771   0.8923479
      0.0104930   0.2709021  -1.4985133
```

## REFERENCES


[1] G. Grell, O. Kühn, and S. I. Bokarev, Phys. Rev. A **100**, 042512 (2019).

[2] A. Kivimäki, M. Neeb, B. Kempgens, H. M. Köppe, and A. M. Bradshaw, J. Phys. B At. Mol. Opt. Phys. **29**, 2701 (1996).

[3] G. Bieri and L. Åsbrink, J. Electron Spectrosc. Relat. Phenom. **20**, 149 (1979).

[4] T. Åberg, Phys. Rev. **156**, 35 (1967).

[5] K. Ueda, M. Okunishi, H. Chiba, Y. Shimizu, K. Ohmori, K. Sato, E. Shigemasa, and N. Kosugi, Chem. Phys. Let. **236**, 311 (1995).

[6] J. Schirmer, A. B. Trofimov, K. J. Randall, J. Feldhaus, A. M. Bradshaw, Y. Ma, C. T. Chen, and F. Sette, Phys. Rev. A **47**, 1136 (1993).

[7] Y. Ma, C. T. Chen, G. Meigs, K. Randall, and F. Sette, Phys. Rev. A **44**, 1848 (1991).

[8] C. D. Caldwell, S. J. Schaphorst, M. O. Krause, and J. Jiménez-Mier, J. Electron Spectrosc. Relat. Phenom. **67**, 243 (1994).

[9] P.-O. Widmark, P. Å. Malmqvist, and B. O. Roos, Theor. Chim. Acta **77**, 291 (1990).

[10] K. Kaufmann, W. Baumeister, and M. Jungen, J. Phys. B At. Mol. Opt. Phys. **22**, 2223 (1989).

[11] J. Almlöf and P. R. Taylor, J. Chem. Phys. **86**, 4070 (1987).

[12] I. Fernández Galván, M. Vacher, A. Alavi, C. Angeli, F. Aquilante, J. Autschbach, J. J. Bao, S. I. Bokarev, N. A. Bogdanov, R. K. Carlson, L. F. Chibotaru, J. Creutzberg, N. Dattani, M. G. Delcey, S. S. Dong, A. Dreuw, L. Freitag, L. M. Frutos, L. Gagliardi, F. Gendron, A. Giussani, L. González, G. Grell, M. Guo, C. E. Hoyer, M. Johansson, S. Keller, S. Knecht, G. Kovačević, E. Källman, G. Li Manni, M. Lundberg, Y. Ma, S. Mai, J. P. Malhado, P. Å. Malmqvist, P. Marquetand, S. A. Mewes, J. Norell, M. Olivucci, M. Oppel, Q. M. Phung, K. Pierloot, F. Plasser, M. Reiher, A. M. Sand, I. Schapiro, P. Sharma, C. J. Stein, L. K. Sørensen, D. G. Truhlar, M. Ugandi, L. Ungur, A. Valentini, S. Vancoillie, V. Veryazov, O. Weser, T. A. Wesołowski, P.-O. Widmark, S. Wouters,

A. Zech, J. P. Zobel, and R. Lindh, J. Chem. Theory Comput. **15**, 5925 (2019).
